# Supplementary material for: RT-Counter: Real-Time Text-Guided Open-Vocabulary Object Counting
Source: arXiv:2606.17561 source file (2026-06-16)
Supplement: Supplementary file 1 [file X_suppl.tex]

\clearpage
\setcounter{page}{1}
\maketitlesupplementary

\section{Training Details}
\paragraph{Hardware Environment:} All experiments are conducted on a workstation equipped with an NVIDIA RTX 3090 GPU and an AMD EPYC 7601 CPU, providing sufficient computational resources for training and evaluation.

\paragraph{Software Environment:} We implement our RT-Counter framework using PyTorch 2.0 with CUDA 11.8 support for GPU acceleration and optimized tensor operations.

\paragraph{Hyper-parameters:} In the optimization of the loss function, the hyperparameters are set as follows: \(\lambda_1 = 0.25\), \(\lambda_2 = 5\), $S=4$, \(\phi=0.5\), \(\sigma=0.5\), and \(N_p=16\). According to \cite{P2PNet}, anchor points are generated at every two-pixel interval in the original image, with each anchor placed at the center of the respective pixel. 

\paragraph{Model Details:}
Our RT-Counter framework is built upon the YOLO-E architecture in \cite{yoloe}, specifically utilizing YOLO-E-11s aligned weights as the backbone for efficient visual feature extraction. For text encoding, we employ the MobileCLIP-BLT model in \cite{mobileclip}, which provides lightweight yet effective textual representation learning while maintaining computational efficiency. During the inference pipeline, object categories are pre-configured and their corresponding textual embeddings are computed and saved as .pt files. During actual inference, the model loads these pre-computed category encodings from the .pt files, eliminating the need for real-time text encoding and significantly reducing the computational overhead. This design choice enables a faster inference speed while maintaining the flexibility of text-guided counting across different object categories.

\begin{figure}[h]
    \centering
    \includegraphics[width=0.9\linewidth]{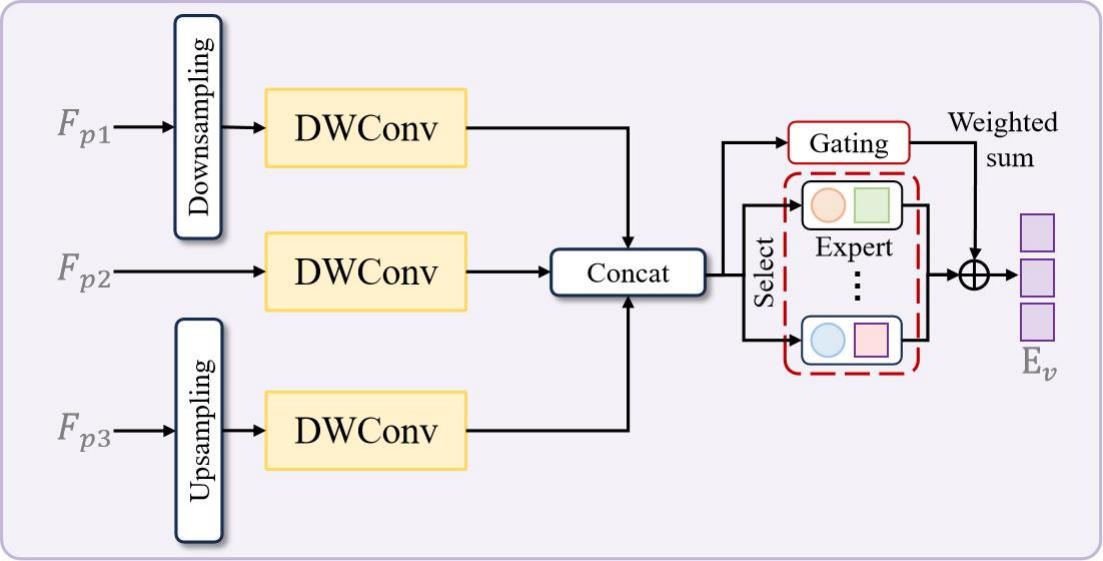}
    \caption{The architecture of the embedding module. Multi-scale features ($F_{p1}$, $F_{p2}$, and $F_{p3}$) are first unified to a common resolution and refined by DWConv layers. The concatenated features are then fed into a Mixture-of-Experts (MoE) network. A Gating mechanism dynamically computes weights for multiple parallel Expert networks. The final output, $E_v$, is produced by a weighted sum of the expert outputs, enabling an adaptive and powerful feature fusion.}
    \label{fig:mgf}
\end{figure}
\section{Supplementary Component Architecture}
\paragraph{Visual embedding module:}
\label{sec:mgf}
To effectively handle objects of various sizes and appearances, we introduce the visual embedding module, as illustrated in Figure~\ref{fig:mgf}. This module is designed to adaptively fuse features from different levels of the feature Path Aggregation Network (PAN) ($F_p$). 

The input to the visual embedding module consists of three feature maps from different scales: a high-resolution map $F_{p1}$, a medium-resolution map $F_{p2}$, and a low-resolution map $F_{p3}$. To create a unified representation, we first bring them to a common resolution of $\frac{H}{16} \times \frac{W}{16}$. This is achieved by applying a strided convolution for {downsampling} $F_{p1}$ and a bilinear interpolation for {upsampling} $F_{p3}$, while $F_{p2}$ remains unchanged.

Each of the scale-aligned feature maps is then processed by a lightweight DWConv to refine its spatial features independently. The three refined feature maps are subsequently {concatenated} along the channel dimension, creating a rich, multi-scale feature descriptor.

Instead of using a static fusion method like a simple convolution, we employ a dynamic MoE network to process this concatenated descriptor. The MoE network consists of two main components:
\begin{itemize}
    \item A set of $n$ {Expert} networks, where each expert is a small feed-forward network specialized in learning different types of patterns (e.g., textures, edges, or specific object parts).
    \item A {Gating} network, which is a lightweight router that takes the concatenated features as input and outputs a set of weights (logits) indicating which experts are most suitable for the current input.
\end{itemize}
The final output, the enhanced visual embedding $E_v$, is produced by a {weighted sum} of the outputs from all expert networks, where the weights are determined by the gating network. This MoE-based design allows our model to dynamically select and combine the most relevant feature transformations for any given input, resulting in a highly adaptive and powerful fusion mechanism.

\paragraph{Visual Prototype Textualization (VPT) Motivation:}
Inspired by zero-shot LOCA~\cite{loca1}, we identify a critical challenge: frequent co-occurring visual patterns create ambiguity in open-vocabulary counting. For instance, when counting "apples" in markets, "oranges" appear as distractors; when counting "cars" on highways, "trucks" cause confusion. Existing text-guided methods cannot effectively distinguish targets from these semantically overlapping elements.

We propose the VPT converting high-frequency visual patterns into text feature space for semantic filtering. Specifically, VPT learns visual prototype tokens to capture frequently occurring features, projects them into text-aligned space via FFN, then performs cross-attention with text descriptions. Features with high text-similarity (target-relevant) are retained, while low-similarity high-frequency patterns (semantically irrelevant) are suppressed. This enables semantic-aware filtering of frequent-but-irrelevant distractors, significantly reducing false positives.

\paragraph{Novelty Justification of Weaformer:}
Standard self-attention mechanisms excel at small-scale image classification tasks but struggle with fine-grained tasks like object counting due to their quadratic complexity with respect to input size. To address this computational bottleneck, various efficient attention mechanisms have been proposed, including local attention (e.g., Swin Transformer~\cite{swin}, Contextual Transformer~\cite{CoT}, ESC~\cite{esc}), linear attention (e.g., ReLU Linear Attention~\cite{reluattn}, PolaFormer~\cite{polaformer}, MALA~\cite{MALA}), and downsampling attention (e.g., HiLo~\cite{hiloattn}, Pyramid Pooling Transformer~\cite{P2T}).

While these methods reduce computational complexity, they face fundamental limitations when applied to open-vocabulary object counting. Pure local attention (e.g., Swin) sacrifices global consistency, leading to duplicate counting in crowded scenes. Linear attention methods, though suitable for long sequences, introduce approximation errors that degrade counting accuracy. Downsampling-based approaches (e.g., HiLo) reduce token counts but often lose fine-grained spatial details critical for precise instance localization.

% Weaformer addresses these challenges through a novel prototype-guided token decomposition strategy. 
Weaformer \emph{adaptively} routes tokens into local and global paths. The local path employs Convolution Attention (ConvAttention) with a 3$\times$3 kernel to preserve fine-grained information, while the global path applies downsampled self-attention on only 25\% of tokens to maintain global perception field (global consistency). This content-adaptive decomposition achieves superior accuracy-efficiency trade-offs specifically tailored for counting tasks. 

To validate our design, we conduct ablation studies comparing Weaformer against state-of-the-art efficient attention mechanisms on FSC147 (Table~\ref{tab:weaformer_ablation}). Specifically, we replace either the ConvAttention module in the local path (Swin-Transformer) or the Weaformer layer (all other variants) with alternative attention mechanisms, while keeping VPT and backbone configurations identical. The results reveal several important insights: (1) Swin-Transformer, which preserves our prototype-guided decomposition framework while only modifying the local path, achieves strong test set performance (12.84 MAE), demonstrating the effectiveness of our dual-path design. (2) While individual methods excel in specific metrics—ESC achieves the best validation RMSE (49.93) and ReLU Linear obtains the best test MAE (12.72)—they exhibit poor generalization across splits, with ESC's test RMSE degrading to 115.96 and ReLU Linear's test RMSE reaching 111.65. (3) In contrast, our full Weaformer model achieves the most balanced and consistent performance across both validation and test sets (12.56/13.30 MAE, 51.25/104.63 RMSE), demonstrating superior generalization. This validates that both our ConvAttention design work synergistically to ensure robust counting performance across diverse scenarios, rather than overfitting to specific metrics or data distributions.

\begin{table}[htbp]
\centering
\caption{Ablation study comparing Weaformer with alternative efficient attention mechanisms on FSC147. All variants use identical VPT and backbone configurations.}
\label{tab:weaformer_ablation}
\begin{tabular}{lcccc}
\toprule
\multicolumn{1}{c}{\multirow{2}{*}{\textbf{Attention}}} & \multicolumn{2}{c}{\textbf{FSC-147 Val}} & \multicolumn{2}{c}{\textbf{FSC-147 Test}} \\
\cmidrule(lr){2-3} \cmidrule(lr){4-5}
 & MAE$\downarrow$ & RMSE$\downarrow$ & MAE$\downarrow$ & RMSE$\downarrow$ \\
\midrule
 Swin~\cite{swin} & 13.51 & 53.83 & 12.84 & 108.53 \\
ReLU Linear~\cite{reluattn} & 13.77 & 55.77 & \textbf{12.72} & 111.65 \\
PolaFormer~\cite{polaformer} & 13.57 & 53.06 & 13.87 & 110.19 \\
MALA~\cite{MALA} & 13.59 & 54.97 & 13.84 & 110.92 \\
ESC~\cite{esc} & 13.59 & \textbf{49.93} & 14.42 & 115.96 \\
\midrule
\textbf{Weaformer (Ours)} & \textbf{12.56} & 51.25 & 13.30 & \textbf{104.63} \\
\bottomrule
\end{tabular}
\end{table}

Second, we analyze the impact of global-local token allocation ratios in Table~\ref{tab:token_ratio}. We experiment with three configurations: balanced allocation (1:1, 50\% tokens to each path), global-dominant (3:1, 75\% global / 25\% local), and local-dominant (1:3, 25\% global / 75\% local). The results demonstrate that the 1:3 ratio (our default setting) achieves the best performance across all metrics. The balanced 1:1 allocation yields suboptimal results (13.39 MAE, 57.77 RMSE on validation), suggesting that equal distribution prevents either path from fully leveraging its specialized capabilities. Interestingly, the 3:1 global-dominant configuration performs even worse (13.53 MAE, 55.25 RMSE on validation), indicating that over-reliance on downsampled global attention sacrifices critical fine-grained spatial details necessary for accurate instance localization. In contrast, our 1:3 local-dominant design allocates 75\% tokens to ConvAttention for detailed boundary preservation while reserving 25\% for global context modeling, achieving optimal counting accuracy (12.56 MAE, 51.25 RMSE on validation). 
% This demonstrates that open-vocabulary counting primarily benefits from fine-grained local processing guided by prototypes.%, with selective global attention serving as a complementary mechanism to ensure scene-level consistency. %The superior performance of our asymmetric allocation validates the design principle that local detail preservation should dominate, while global reasoning provides essential regularization against duplicate counting.

\begin{table}[htbp]
\centering
\caption{Ablation study on local-global token allocation ratios in Weaformer. The ratio represents Local:Global token distribution.}
\label{tab:token_ratio}
\begin{tabular}{ccccc}
\toprule
\multicolumn{1}{c}{\multirow{2}{*}{\textbf{Global : Local}}} & \multicolumn{2}{c}{\textbf{FSC-147 Val}} & \multicolumn{2}{c}{\textbf{FSC-147 Test}} \\
\cmidrule(lr){2-3} \cmidrule(lr){4-5}
 & MAE$\downarrow$ & RMSE$\downarrow$ & MAE$\downarrow$ & RMSE$\downarrow$ \\
\midrule
1:1& 13.39 & 57.77 & \textbf{13.21} & 110.13 \\
3:1& 13.53 & 55.25 & 13.31 & 111.11 \\
\midrule
\textbf{1:3} & \textbf{12.56} & \textbf{51.25} & 13.30 & \textbf{104.63} \\
\bottomrule
\end{tabular}
\end{table}

\paragraph{Detailed Description of ConvAttention:}
\label{sec:supp_convattention}
The {Convolutional Attention (ConvAttention)} block is a core component of our Weaformer layer, designed to efficiently capture local features by emulating the inductive biases of convolution within an attention framework. Unlike standard self-attention that computes global relationships with quadratic complexity, ConvAttention operates on local windows with linear complexity. The detailed mechanism is illustrated in the main paper and described below.

\textbf{Projection via DWConv:}
Given an input feature map $X \in \mathbb{R}^{B \times D \times H' \times W'}$, we first generate the query ($Q$), key ($K$), and value ($V$) tensors. Instead of using standard $1\times 1$ convolutions, we employ efficient {Depth-wise Convolutions (DWConv)}. This choice is deliberate as DWConv processes each channel independently, which is computationally efficient and preserves channel-specific spatial patterns, analogous to how grouped convolutions operate.
\begin{equation}
    [Q, K, V ]= \text{DWConv}(X)
\end{equation}

\textbf{Local Window Construction via Unfold:}
To enforce locality, the attention computation is constrained to a local window of a predefined size, e.g., $k \times k$. This is achieved by applying the unfold operation, which extracts sliding local blocks from a tensor. As depicted in the diagram, this operation is applied to the query tensor $Q$, transforming it from a feature map into a collection of patches or ``local windows''.
\begin{equation}
    Q_{patches} = \text{unfold}(Q) \in \mathbb{R}^{B \times (D k^2) \times (H' W')}
\end{equation}
To maintain alignment, the same {unfold} operation is conceptually applied to the key ($K$) and value ($V$) tensors, creating corresponding local patches $K_{patches}$ and $V_{patches}$ for each query window.

\begin{figure}
    \centering
    \includegraphics[width=\linewidth]{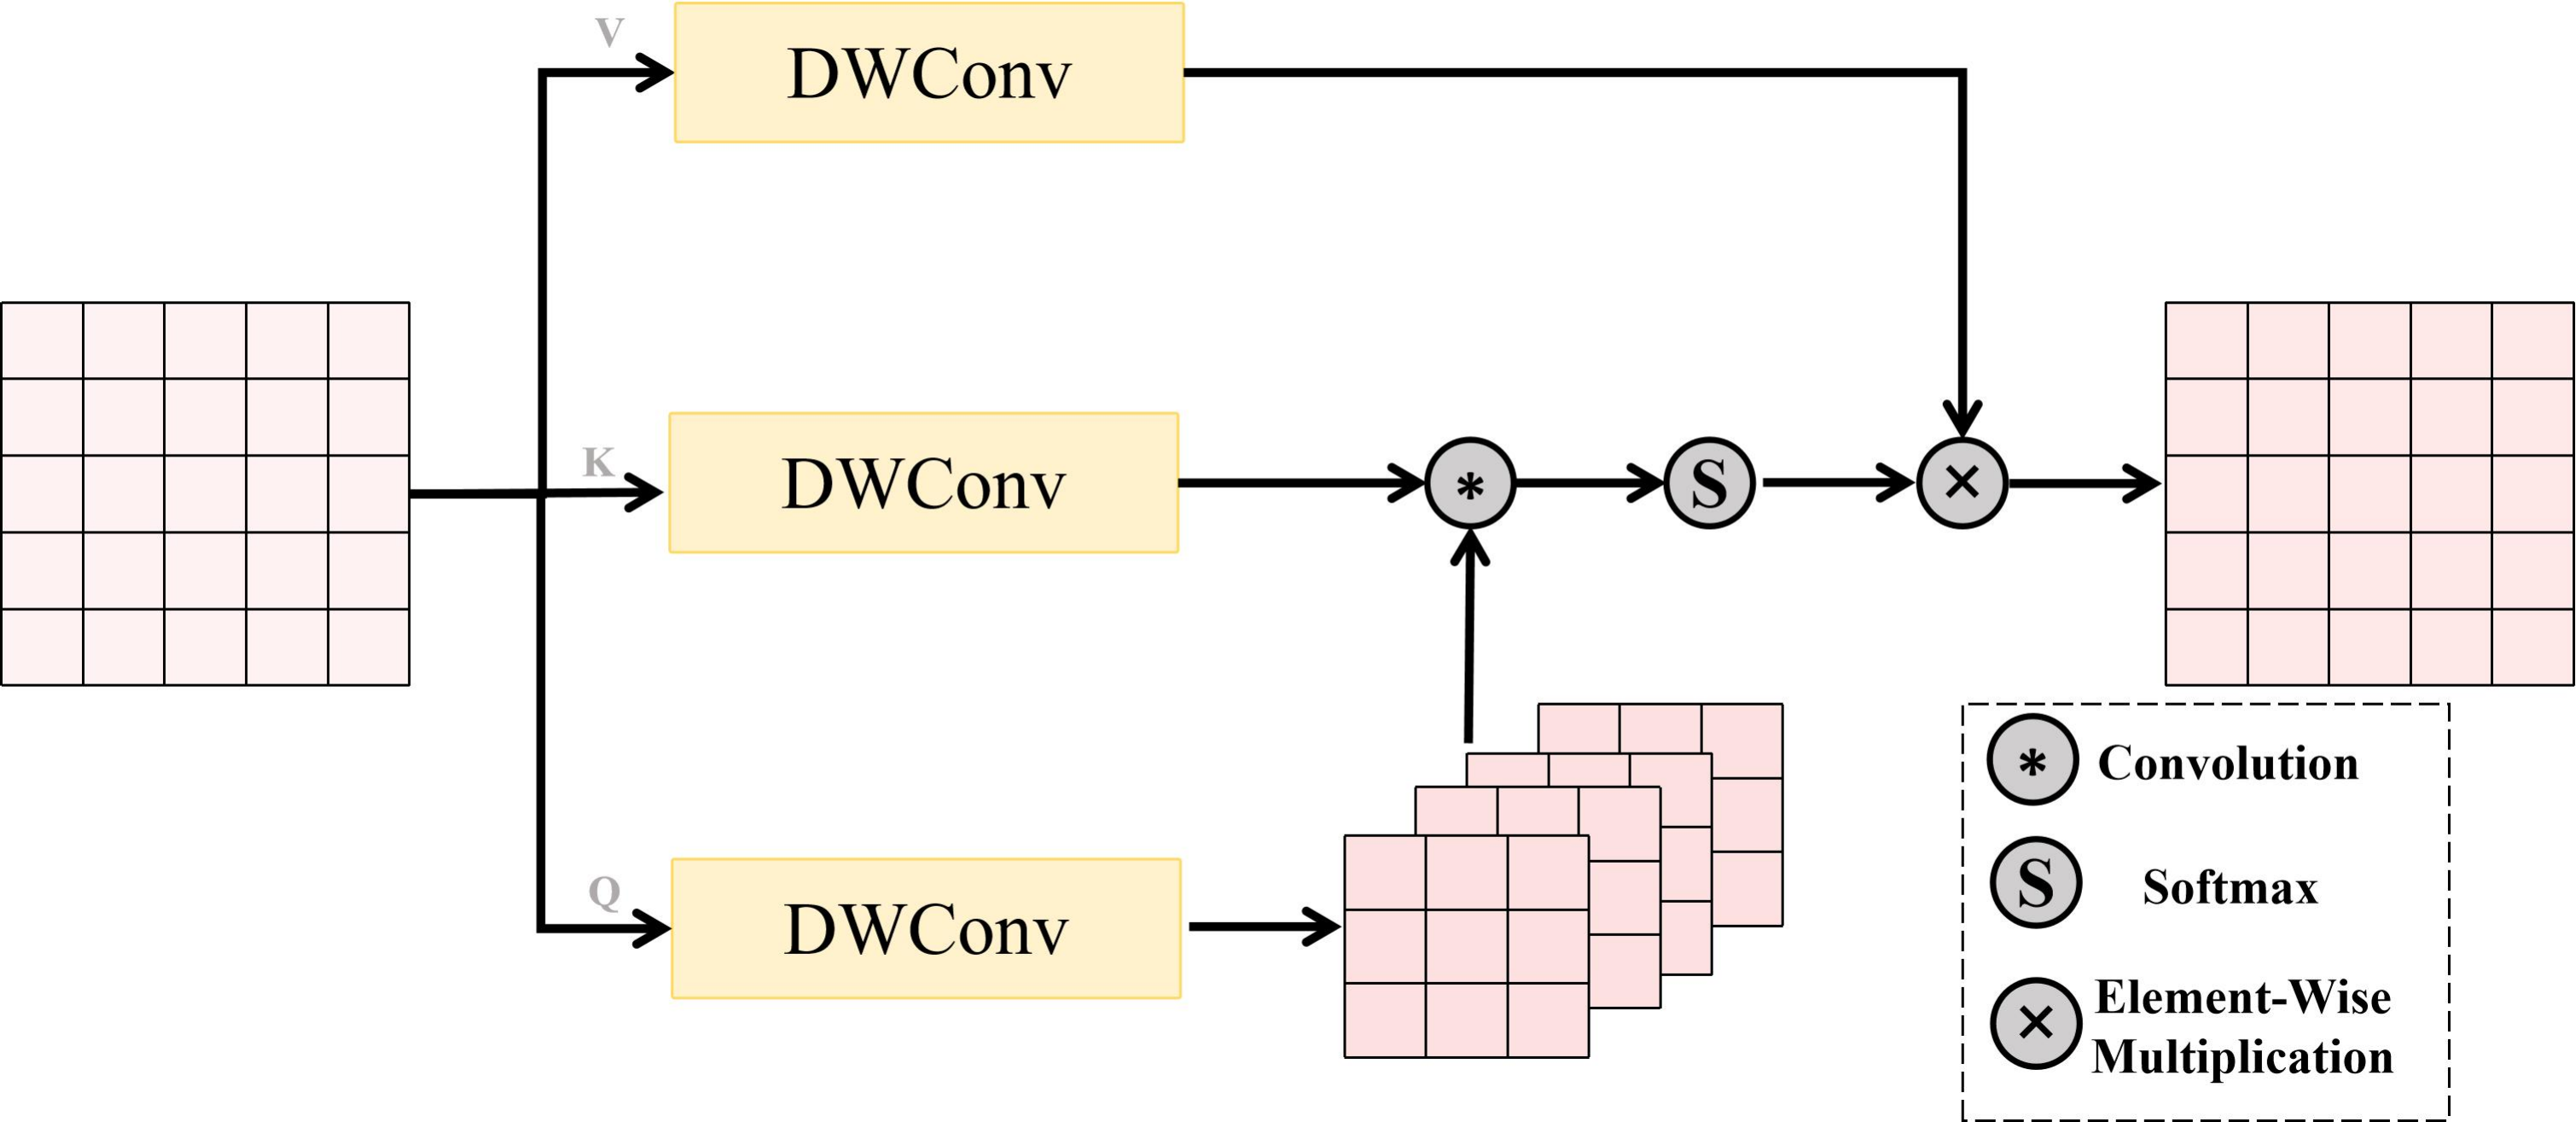}
    \caption{Architecture of our proposed Convolutional Attention (ConvAttention) block.}
    \label{fig:convattn}
\end{figure}

\textbf{Attention as a Dynamic Convolution Kernel:}
The most novel aspect of ConvAttention is how it simulates a convolution. Here, the key tensor $K$ is dynamically reshaped to act as the convolution kernel weights. The attention mechanism computes the similarity between the local query patches ($Q_{patches}$) and the corresponding local key patches ($K_{patches}$). As shown in the diagram, this interaction can be an element-wise product ($\ast$), which computes the attention scores ($\text{AttentionScores}$) for each position within the local window. Namely, 
\begin{equation}
	 \text{AttentionScores} = Q_{patches} \ast K_{patches} 	
\end{equation}
These scores are then normalized via a Softmax function to form the attention weights, which effectively act as a dynamic, data-dependent convolution kernel. That is, 
\begin{equation}
	\text{AttentionWeights} = \text{softmax}(\text{AttentionScores})         
\end{equation}

\textbf{Weighted Sum for Output:}
The learned AttentionWeights are used to perform a weighted sum of the value patches ($V_{patches}$). This operation is analogous to the multiplication and summation step in a standard convolution, where the output for a central position is an aggregation of its neighbors, weighted by the learned kernel. The final output is obtained by folding these aggregated patch features back into a feature map of the original spatial dimensions using the {fold} operation. That is,
\begin{equation}
    O_{local} = \text{fold}(\text{AttentionWeights} \otimes V_{patches})
\end{equation}
where $\otimes$ means the element wise multiplication.

In summary, the ConvAttention module ingeniously combines the efficiency of DWConv and the local processing of the {unfold} operation with a dynamic weighting mechanism inspired by self-attention. This allows it to function as a highly efficient and data-dependent version of a standard convolution, making it a perfect component for the local feature extraction path within our Weaformer.

\paragraph{Prediction Head:} The enhanced features $F_{en}$ are processed through the lightweight prediction head consisting of three convolutional layers with ReLU activations. That is, 
\begin{equation}
\text{Output} = \text{Conv}_2(\text{BN}(\text{ReLU}(\text{Conv}_1(F_{en})))
\end{equation}
Each convolutional layer employs Conv\&ReLU operations to generate final predictions for object locations and confidence scores, enabling the efficient end-to-end training and inference.

\paragraph{Auxiliary Network Architecture:}

The auxiliary network uses a residual SwiGLU-FFN design
\begin{equation}
    E_{t} = E_{t'} + \text{SwiGLU}(\text{FFN}(E_{t'}))
\end{equation}
We choose \text{SwiGLU} over standard activations.

\begin{figure}[ht]
    \centering
    \includegraphics[width=\linewidth]{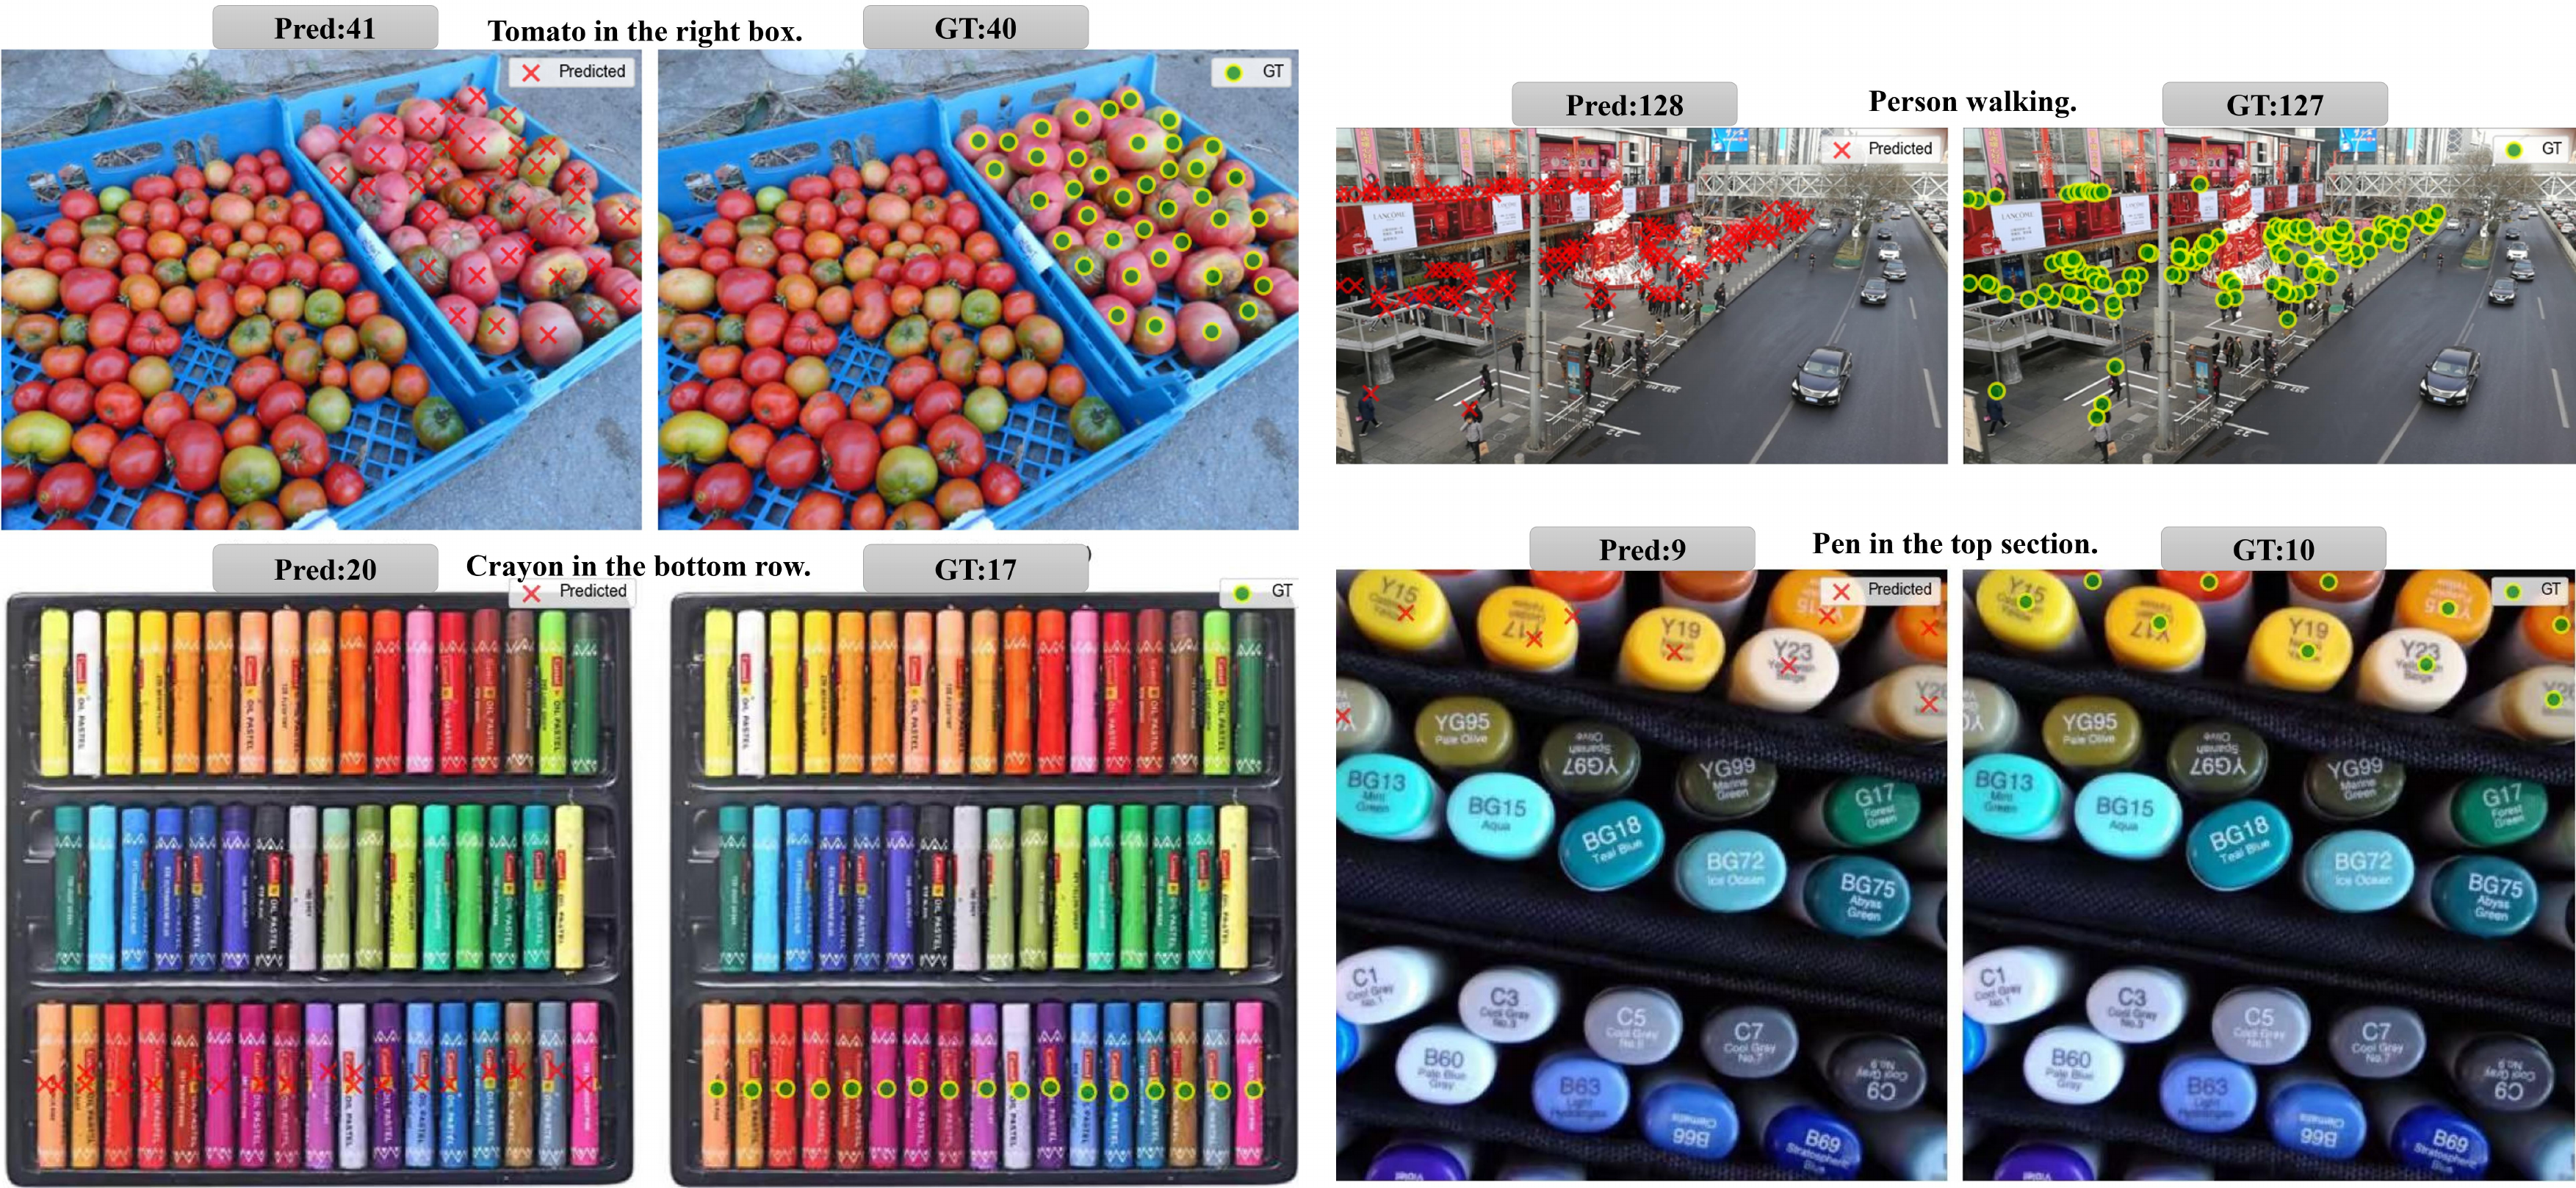}
    \caption{Qualitative results on the REC8K dataset. The model has the accurate counting and localization performance under various referring expressions. It can effectively understand text-guided spatial semantics such as “in the right box”, “walking person”, “in the bottom row”, and “in the top section”. Minor deviations are mainly caused by occlusion and ambiguous semantic boundaries.}
    \label{fig:recres}
\end{figure}

\section{Supplemental visualization results}
\paragraph{Qualitative results on the REC8K:}
Figure \ref{fig:recres} shows the qualitative results on the REC8K dataset.
The model demonstrates its strong performance in understanding text-guided visual semantics and accurately localizing the referred objects across various scenes.
For example, in “Tomato in the right box” and “Person walking”, the predicted counts 41 and 128 respectively closely match the ground truths 40 and 127, showing the model’s robustness and precise object discrimination even in dense or cluttered environments.
In “Crayon in the bottom row” and “Pen in the top section”, the model effectively captures the spatial and contextual cues indicated by the textual expressions, though minor false detections or omissions occur due to semantic ambiguity and object occlusion.
Overall, these results confirm the effectiveness of the proposed approach in modeling image-text fusion features for referring expression counting.
\begin{figure}[ht]
    \centering
    \includegraphics[width=\linewidth]{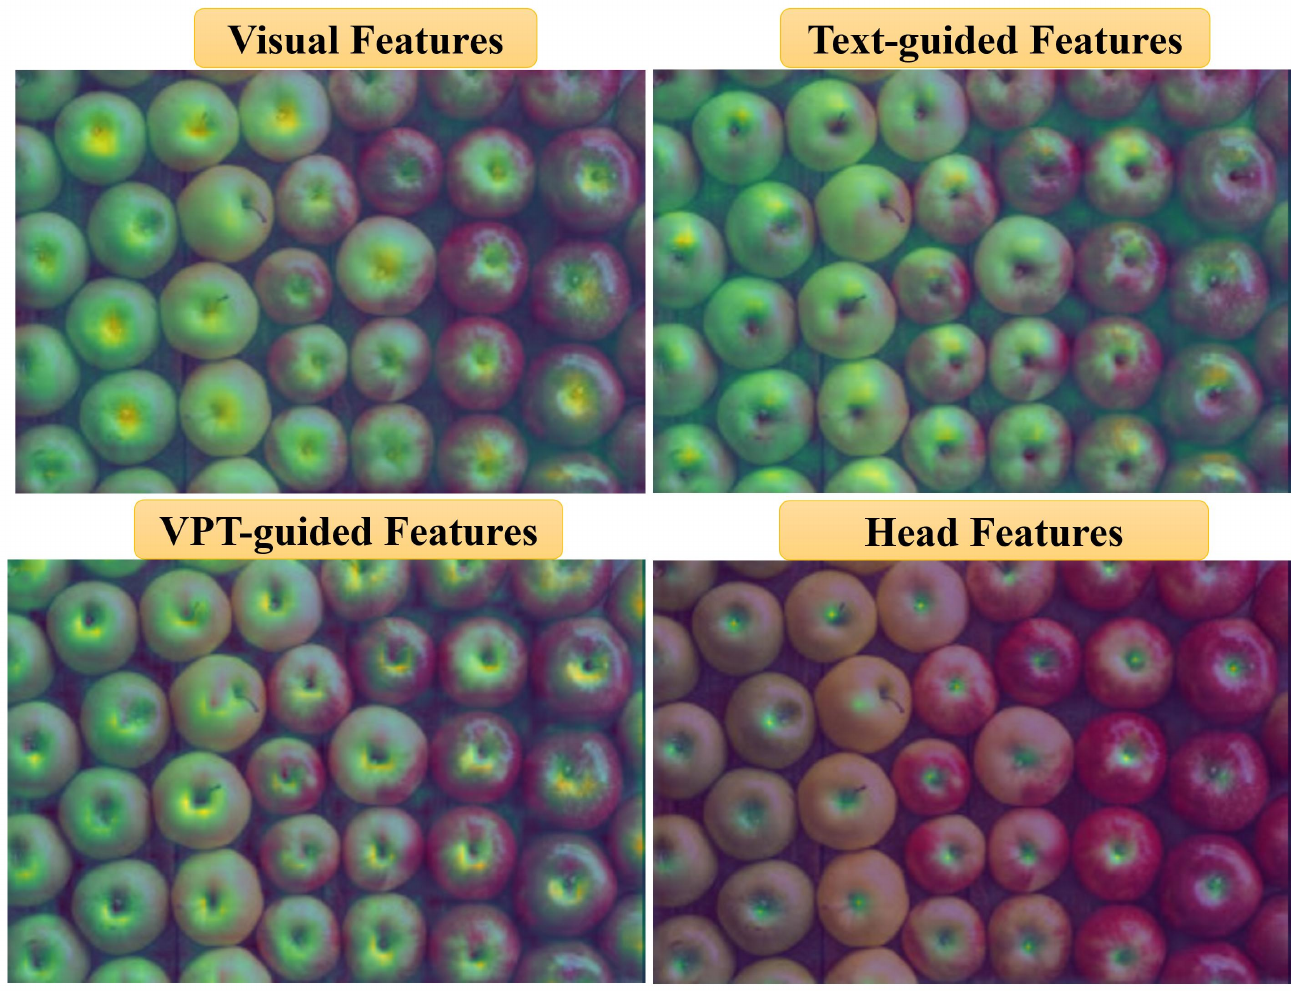}
    \caption{Visualization of different feature representations in the proposed model. 
    From left to right and top to bottom: (a) visual features, (b) text-guided features, 
    (c) VPT-guided features, and (d) head features. 
    The visualization shows that text and VPT guidance progressively refine the activation 
    regions, enabling the model to better focus on the referred targets.}
    \label{fig:feature}
\end{figure}

\begin{figure*}[t]
\centering
\includegraphics[width=\linewidth]{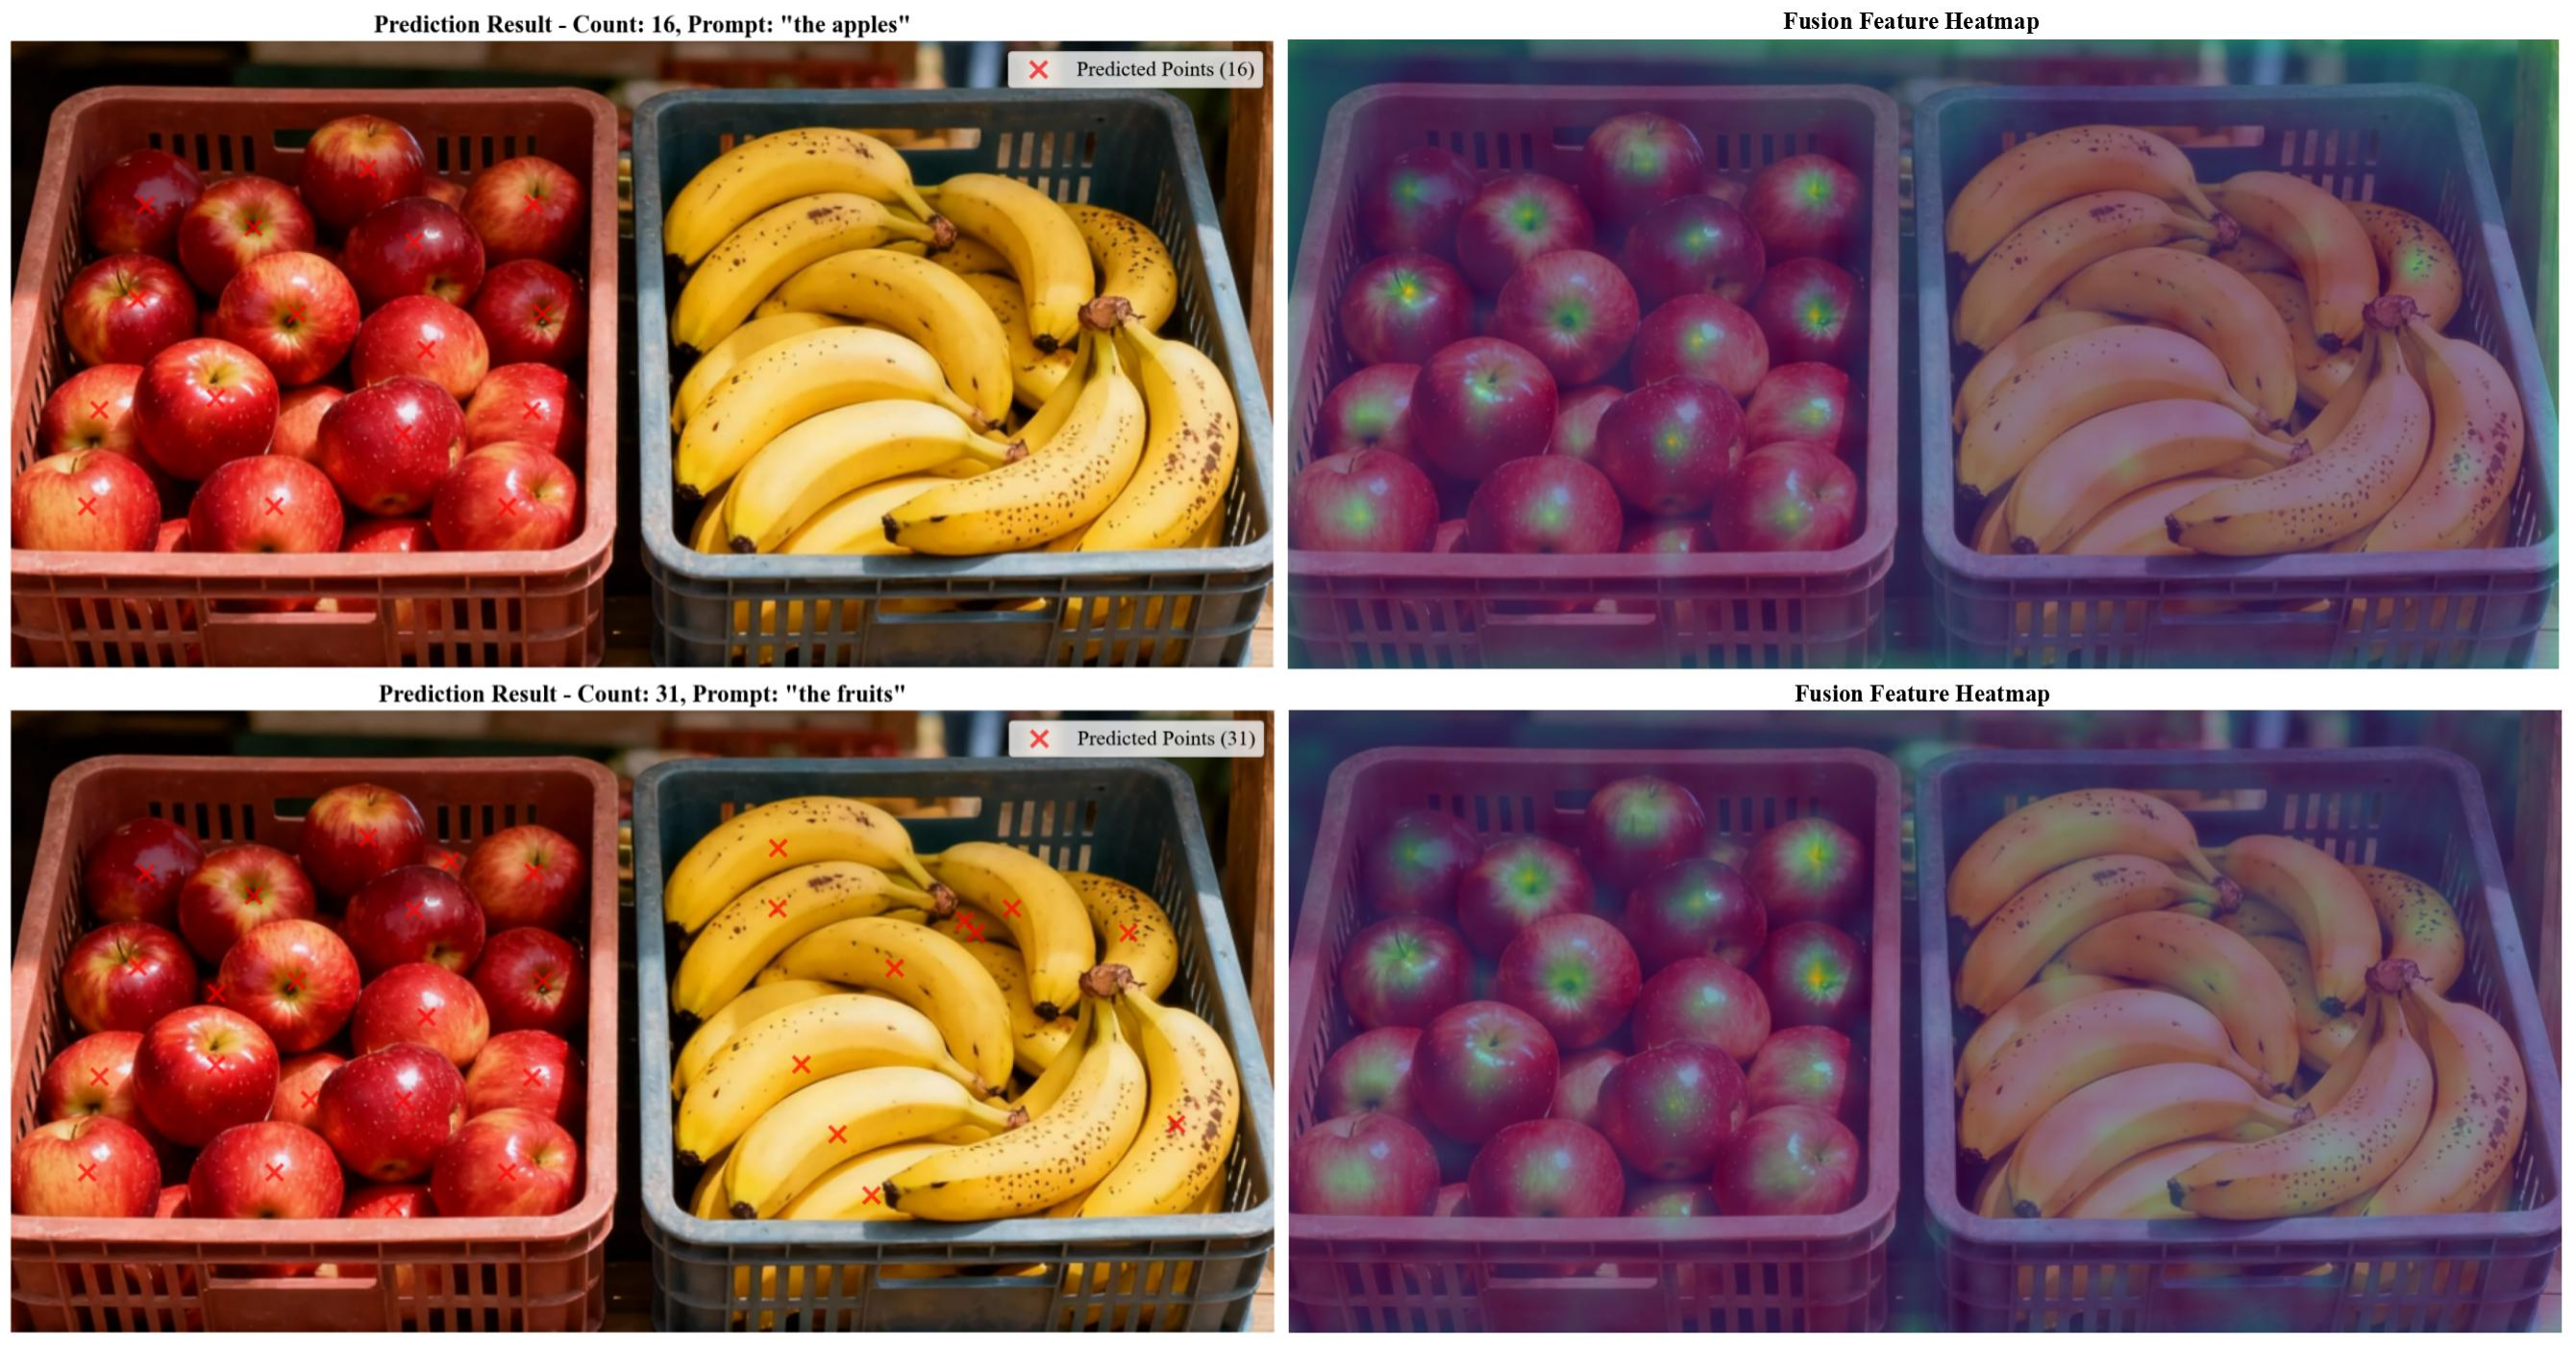}
\caption{VPT Semantic Filtering Visualization. Left: Original images with prediction results. Right: Attention heatmaps after Visual Prototype Textualization. Top row shows specific counting ("the apples", count=16) where bananas are suppressed. Bottom row shows general counting ("the fruits", count=31) where both categories are retained.}
\label{fig:vpt_visualization}
\end{figure*}
\paragraph{Visualization of feature representations:}
Figure \ref{fig:feature} visualizes the feature activation maps from different stages of the proposed model, including visual features, text-guided features, VPT-guided features, and head features.
The visual features primarily capture the low-level object regions, focusing on general color and texture information.
After text guidance, the attention becomes more concentrated on the regions relevant to the referring expression, indicating the effectiveness of text-guided fusion in aligning visual and linguistic modalities.
The VPT-guided features further enhance spatial localization by integrating both visual priors and textual semantics, producing sharper and more discriminative activation maps.
Finally, the head features show refined responses that precisely correspond to the referred targets, confirming that the proposed fusion and guidance mechanisms effectively improve the model’s discriminative capability and cross-modal understanding.

\begin{figure}[ht]
    \centering
    \includegraphics[width=\linewidth]{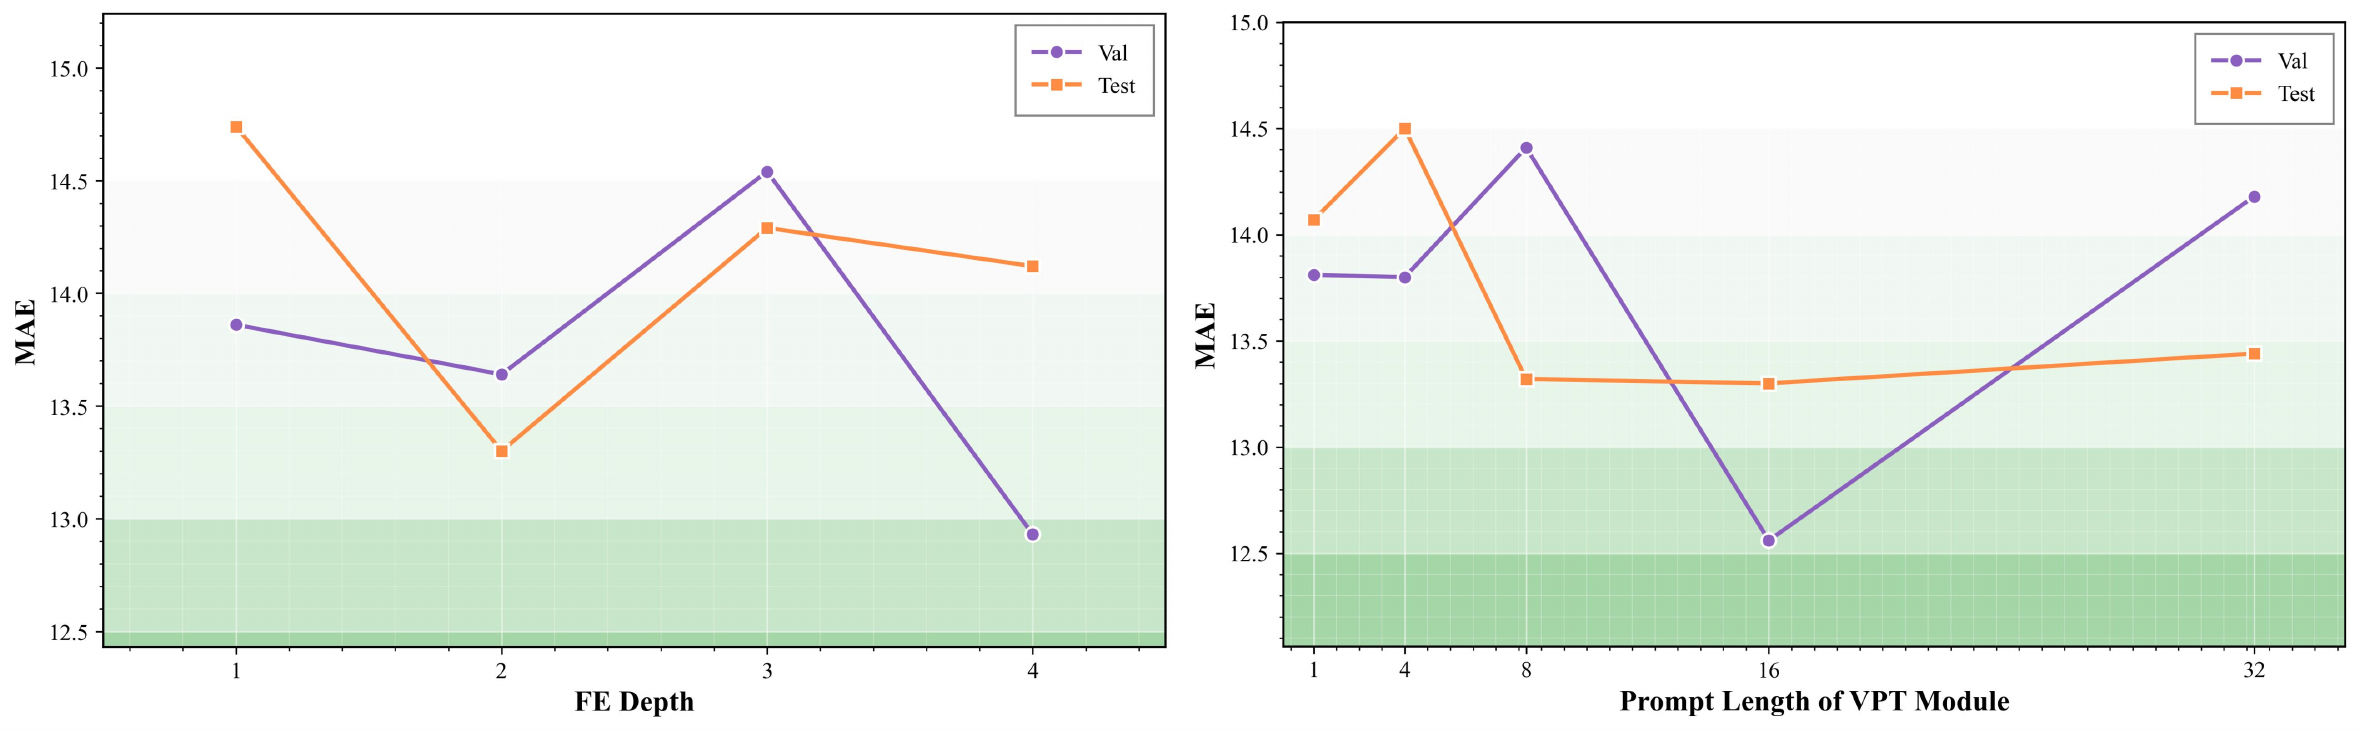}
    \caption{Ablation analysis of the depth of feature extractor (FE) and the number of experts. 
    In the left, increasing the depth of FE improves representation capability up to a moderate level (depth = 2), after which overfitting causes a slight increase in MAE. 
    In the right, expanding the length of prompt enhances the model generalization up to 16, 
    while excessive prompt length introduce redundancy and lead to minor performance degradation.}
    \label{fig:ablation_fe}
\end{figure}

\paragraph{Qualitative Analysis of Semantic Filtering.}
Figure~\ref{fig:vpt_visualization} demonstrates VPT's ability to perform semantic-aware filtering through Visual Prototype Textualization. We visualize the counting results for two text prompts—"the apples" (specific target) and "the fruits" (general category)—on an image containing both apples and bananas.

\textbf{Top row (Prompt: "the apples"):} When querying for a specific object class, VPT correctly identifies 16 apples in the left basket while completely ignoring the bananas in the right basket. The visualization (right panel) shows that learned visual prototypes, after textualization into the embedding space of text, successfully suppress banana-related high-frequency features through cross-attention with the text "apples.".
% The green highlighted regions indicate retained target-relevant features, while banana areas remain unactivated, demonstrating precise semantic discrimination.

\textbf{Bottom row (Prompt: "the fruits"):} When the text prompt becomes more general, VPT adapts its filtering strategy accordingly. The predicted count of 31 objects (16 apples and 15 bananas) shows that the model now retains both fruit categories. The attention map (right panel) reveals that visual prototypes textualized with "the fruits" preserve high-frequency features from both baskets, as both semantically align with the broader category. 
% Red crosses mark all detected instances, confirming that VPT dynamically adjusts its "frequent-but-irrelevant" filtering based on text semantics.

% \textbf{Key Observations:} (1) Visual prototypes learn task-agnostic high-frequency patterns (both apples and bananas are statistically frequent in this image), but their retention/suppression is determined by text-alignment after textualization. (2) The same visual feature (e.g., banana shape/color) is suppressed under "the apples" but retained under "the fruits," validating our semantic-aware filtering mechanism. (3) VPT avoids false positives from visually similar co-occurring objects (apples vs. bananas) without requiring category-specific training, demonstrating robust open-vocabulary generalization.

\paragraph{Visualization of failure cases:}
Figure~\ref{fig:failure_cases} illustrates two representative failure scenarios of our RT-Counter framework. In the top example, our method predicts 100 hot air balloons while the ground truth is 113, demonstrating challenges in counting extremely small objects that blend into complex backgrounds. The balloons in the distant sky appear as tiny colored dots that are difficult to distinguish from background noise, leading to undercounting.

The bottom example shows a more significant failure case where our model predicts 50 sunglasses instead of the ground truth 22. This failure highlights a fundamental limitation when dealing with abstract counting concepts. The term "glasses" refers to complete eyewear units, each consisting of two lenses, but our model lacks the semantic understanding to group lens pairs into single objects without appropriate visual examples in the exemplar set.

Despite our model's overall strong performance, these failure cases reveal two key limitations: (1) difficulty in detecting extremely small objects that highly blend with complex backgrounds, and (2) challenges in handling abstract semantic concepts that require compositional understanding beyond simple visual pattern matching. These limitations suggest future directions for improving semantic reasoning capabilities and enhancing detection of small-scale objects in cluttered environments.
\begin{figure}[ht]
    \centering
    \includegraphics[width=\linewidth]{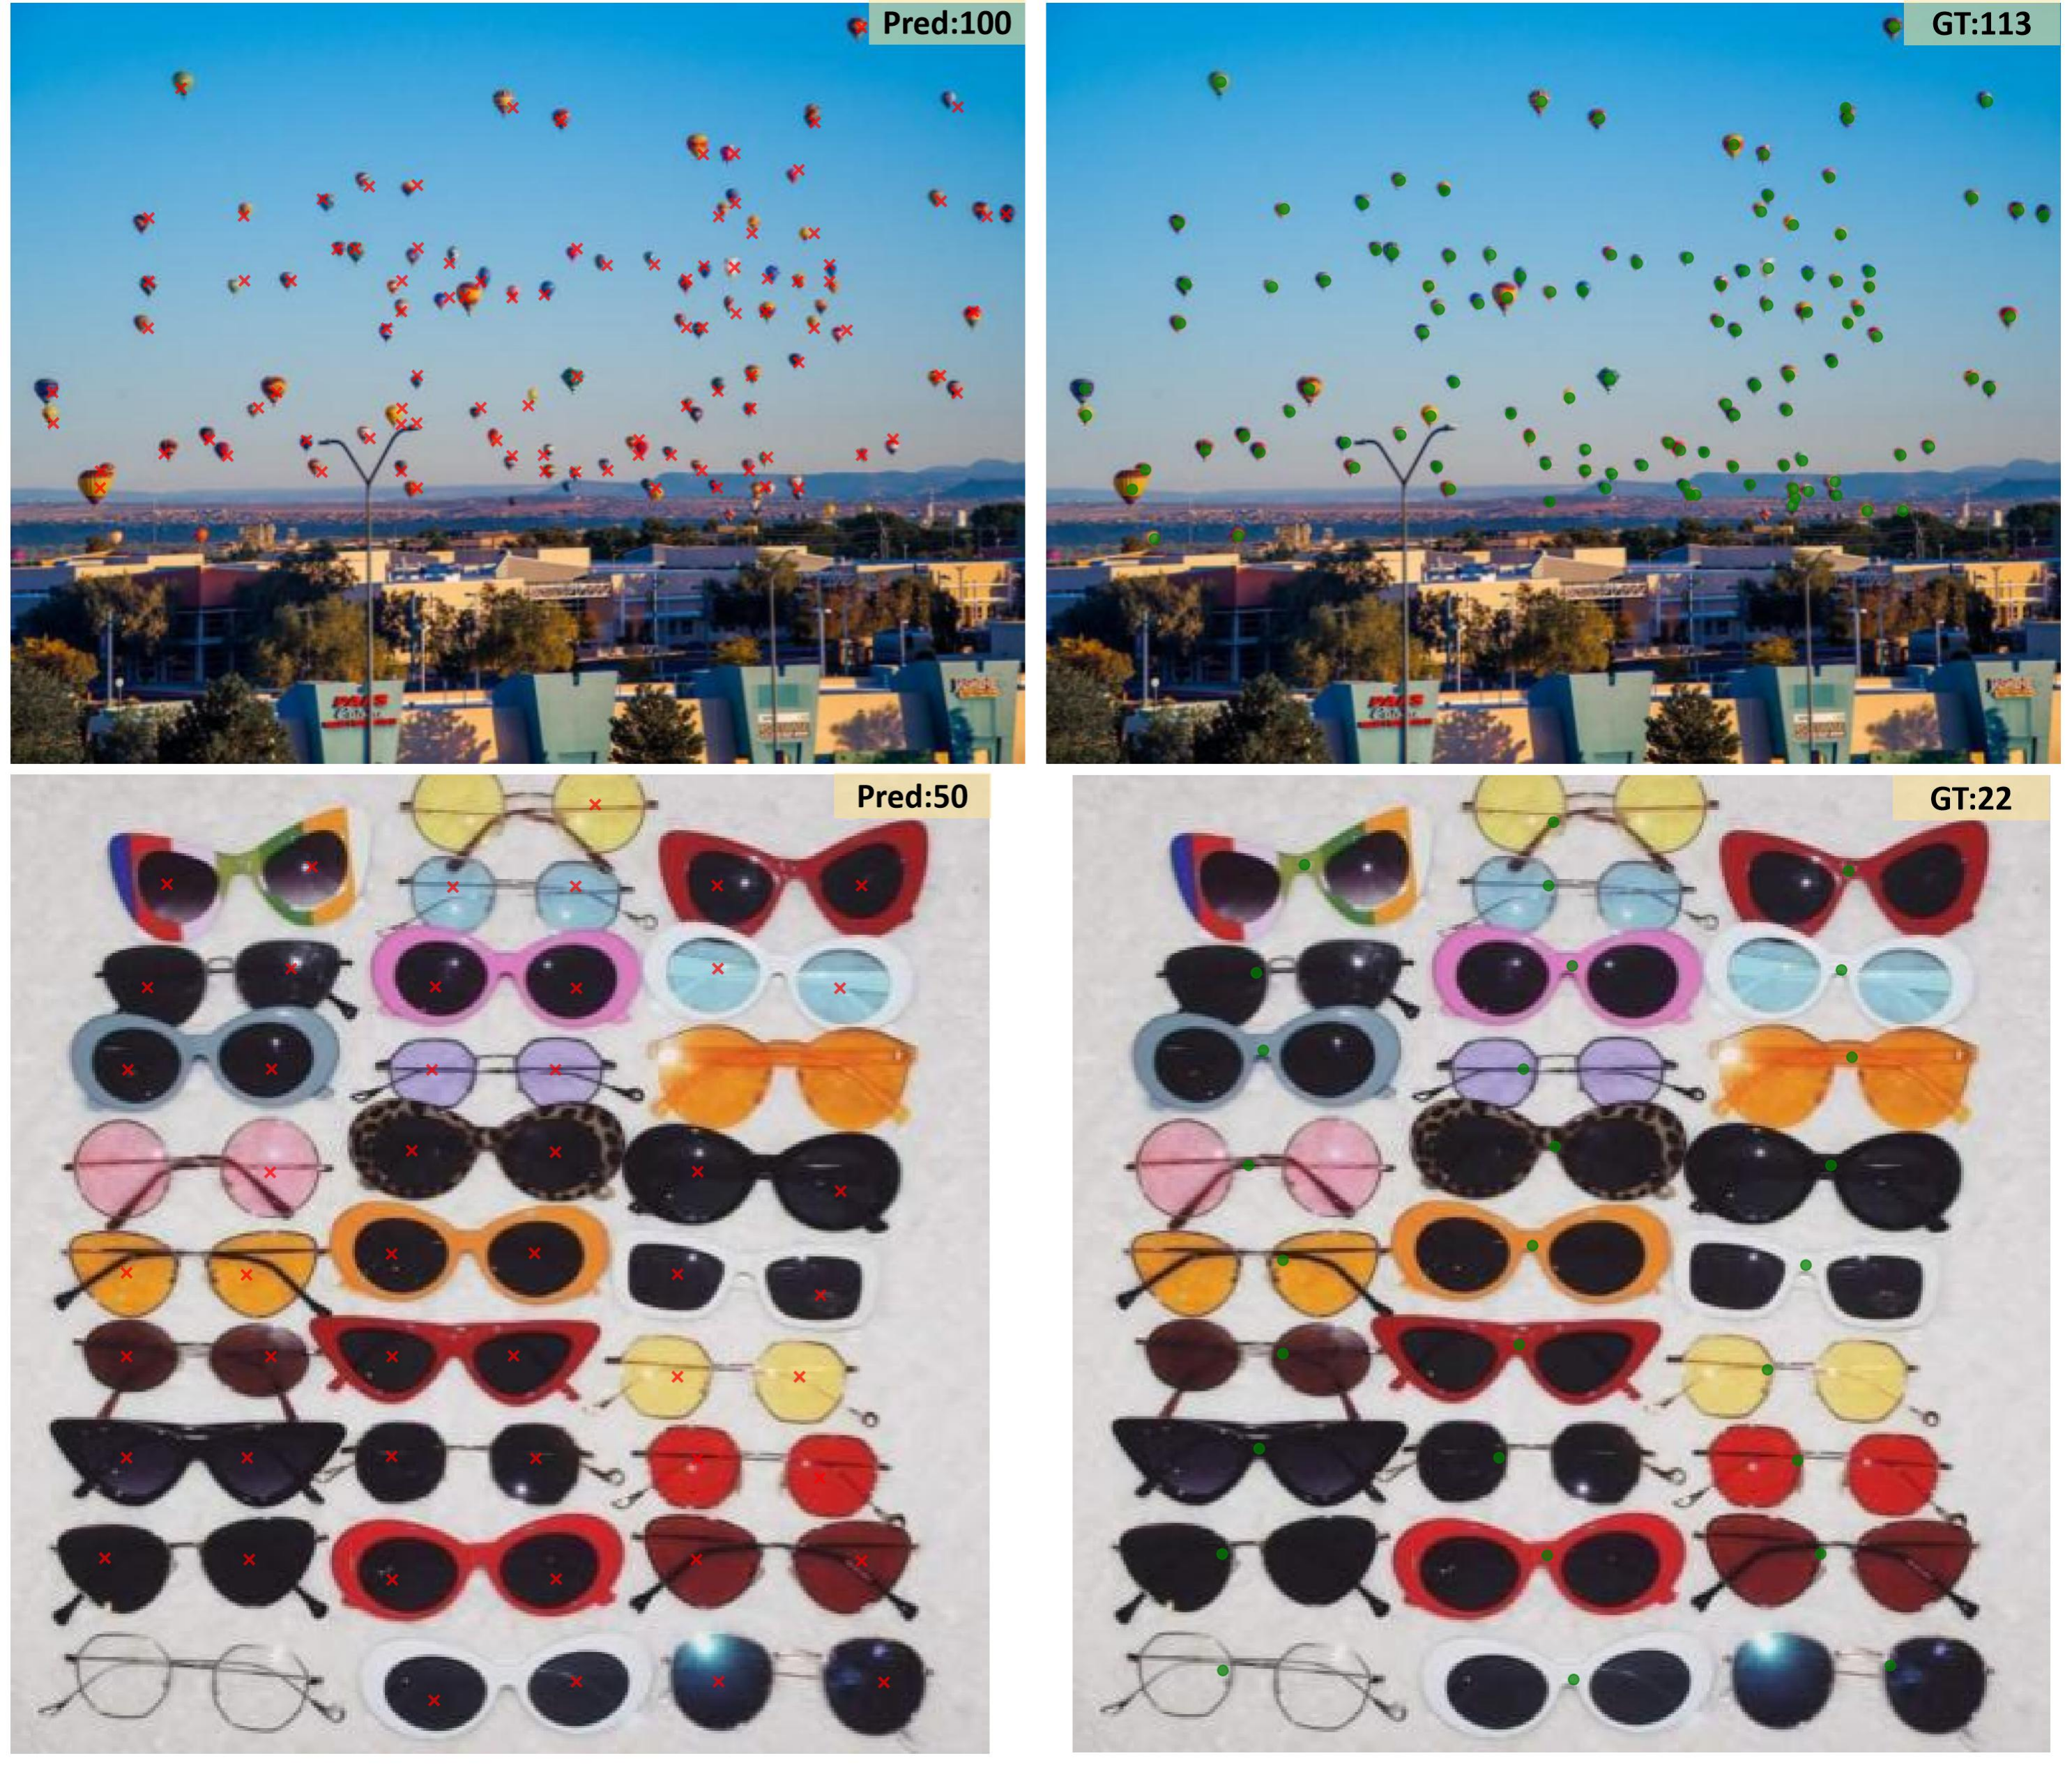}
    \caption{Failure case analysis of RT-Counter. Top: Hot air balloon counting showing under counting of small distant objects (Pred: 100, GT: 113). Bottom: Sunglasses counting demonstrating semantic misunderstanding where individual lenses are counted rather than complete eyewear units (Pred: 50, GT: 22). }
    \label{fig:failure_cases}
\end{figure}
\section{Supplementary Experiment}
\paragraph{Ablation Study on Feature Enhancer Depth and the Length of the Prompt in VPT Module:}
Figure \ref{fig:ablation_fe} gives the ablation study on the depth of the Feature Enchancer (FE) and the length of the prompt in the VPT module. The FE depth is determined by the number of modules, where each depth unit consists of one Weaformer block and one Transformer layer.

In the left plot, the MAE on the validation and test first decrease and then increase as the FE depth grows, indicating that a moderate depth (e.g., depth = 2) achieves the best balance between feature representation and overfitting.
When the FE becomes too deep (depth $\geq$ 3), the model tends to overfit the training data, resulting in performance degradation.

In the right plot, the MAE of the model varies with the length of the prompt $N_p$. Increasing the length of prompt from 4 to 16 improves performance by allowing for more diverse feature specialization, leading to better generalization on both validation and test sets.
However, beyond 16, the performance decreases slightly, which may be due to redundant prompt interactions and reduced parameter efficiency.

Overall, these results demonstrate that an FE depth of 2 and 16 prompt lengths provides the optimal configuration to balance the complexity of the model and generalizability.

\begin{table}[t]
\centering
\caption{Training and inference time required for one epoch on the REC-8K dataset.}
\label{tab:efficiency}
\begin{tabular}{lcc}
\toprule
\textbf{Method} & \textbf{Training Time $\downarrow$} & \textbf{Inference Time $\downarrow$} \\
\midrule
GroundingREC & 54.8  & 6.8 \\
\textbf{RT-Counter (Ours)} & \textbf{7.1 } & \textbf{1.7 } \\
\bottomrule
\end{tabular}
\end{table}

\paragraph{Computational Efficiency:}
To further demonstrate the computational efficiency of our proposed framework, we compare its training and inference times against a recent baseline, GroundingREC. The results, measured per epoch on the REC-8K dataset, are presented in Table~\ref{tab:efficiency}.

The comparison reveals a substantial advantage for our RT-Counter. In terms of training, RT-Counter requires only 7.1 minutes per epoch, which is approximately 7.7 times faster than GroundingREC requiring the 54.8 minutes. The efficiency gain is also pronounced during inference, where our model takes just 1.7 minutes, marking a 4.0 $\times$ speedup over the baseline. This substantial improvement in both training and inference efficiency is a direct result of our architectural design, particularly the replacement of standard self-attention with the highly efficient Weaformer layer. These findings validate that RT-Counter is not only highly accurate but also a practical and scalable solution suitable for real-time applications.

% \section{Rationale}
% \label{sec:rationale}
% % 
% Having the supplementary compiled together with the main paper means that:
% % 
% \begin{itemize}
% \item The supplementary can back-reference sections of the main paper, for example, we can refer to \cref{sec:intro};
% \item The main paper can forward reference sub-sections within the supplementary explicitly (e.g. referring to a particular experiment); 
% \item When submitted to arXiv, the supplementary will already included at the end of the paper.
% \end{itemize}
% % 
% To split the supplementary pages from the main paper, you can use \href{https://support.apple.com/en-ca/guide/preview/prvw11793/mac#:~:text=Delete%20a%20page%20from%20a,or%20choose%20Edit%20%3E%20Delete).}{Preview (on macOS)}, \href{https://www.adobe.com/acrobat/how-to/delete-pages-from-pdf.html#:~:text=Choose%20%E2%80%9CTools%E2%80%9D%20%3E%20%E2%80%9COrganize,or%20pages%20from%20the%20file.}{Adobe Acrobat} (on all OSs), as well as \href{https://superuser.com/questions/517986/is-it-possible-to-delete-some-pages-of-a-pdf-document}{command line tools}.
